# Supplementary material for: A benchmark for video-based laparoscopic skill analysis and assessment
Source: arXiv:2602.09927 source file (2026-02-10)
Supplement: Supplementary file 1 [file supplementary.pdf]

# Annotation guidelines

## General instructions

- Each video is rated on four aspects: depth perception, efficiency, bimanual dexterity, and tissue handling.
- Each aspect is independently assessed on a 5-point Likert scale, ranging from 1 (very bad) to 5 (very good).
- For each aspect, task-specific anchor descriptors are provided to define the rating scale.

## Task-specific instructions

### Peg transfer

#### Task description

Six triangular-shaped rubber objects must be transferred from the left to the right side of a pegboard, using two laparoscopic graspers. This means that each object needs to be picked up with the grasper in the left hand, transferred mid-air to the grasper in the right hand, and then placed on an arbitrary peg on the right side of the pegboard. Afterward, the objects must be transferred from the right side back to the left side, picking each object up with the right hand and, after transfer, placing it on a peg with the left hand.

#### Error description

- A triangular object is dropped within the field of view, and it can be retrieved.
- A triangular object is dropped outside the field of view, or it cannot be retrieved.

#### Criteria for exclusion from the dataset

- Task duration > 6 min.

#### Rating scale with anchor descriptors

| Depth perception                                                                                                                                                                                                                                                                 |   |                                                                                                                                                                                                                                                            |   |                                                                                                                                                                                                                                                                         |
|----------------------------------------------------------------------------------------------------------------------------------------------------------------------------------------------------------------------------------------------------------------------------------|---|------------------------------------------------------------------------------------------------------------------------------------------------------------------------------------------------------------------------------------------------------------|---|-------------------------------------------------------------------------------------------------------------------------------------------------------------------------------------------------------------------------------------------------------------------------|
| 1                                                                                                                                                                                                                                                                                | 2 | 3                                                                                                                                                                                                                                                          | 4 | 5                                                                                                                                                                                                                                                                       |
| <ul style="list-style-type: none"><li>• Objects are approached very slowly and missed multiple times</li><li>• Transferring objects from one grasper to the other often requires several attempts</li><li>• Placing the objects takes twice as long as picking them up</li></ul> |   | <ul style="list-style-type: none"><li>• Objects are approached at moderate speed and are not missed</li><li>• Transferring objects from one grasper to the other works at a moderate pace</li><li>• Placing the objects works without any issues</li></ul> |   | <ul style="list-style-type: none"><li>• Objects are approached purposefully and quickly, and they are not missed</li><li>• Transferring objects from one grasper to the other is efficient and fast</li><li>• Objects are not dropped or placed next to a peg</li></ul> |

### *Efficiency*

| 1                                                                                                                                                                                                                                                                                                                          | 2 | 3                                                                                                                                                                                                                                                                                                               | 4 | 5                                                                                                                                                                                                                                                                                                                                               |
|----------------------------------------------------------------------------------------------------------------------------------------------------------------------------------------------------------------------------------------------------------------------------------------------------------------------------|---|-----------------------------------------------------------------------------------------------------------------------------------------------------------------------------------------------------------------------------------------------------------------------------------------------------------------|---|-------------------------------------------------------------------------------------------------------------------------------------------------------------------------------------------------------------------------------------------------------------------------------------------------------------------------------------------------|
| <ul style="list-style-type: none"> <li>• Picking up the first object is unnecessarily delayed</li> <li>• For the transfer, the second grasper only moves toward the object after the first grasper has picked it up</li> <li>• Placing an object is hesitant, and the object needs to be aligned in the process</li> </ul> |   | <ul style="list-style-type: none"> <li>• Picking up the first object is slow but deliberate</li> <li>• Objects are transferred directly from one grasper to the other, without the need to realign them</li> <li>• Objects are placed in a directed manner, with slight alignment movements required</li> </ul> |   | <ul style="list-style-type: none"> <li>• The first object is picked up immediately and without issues</li> <li>• Picking up and placing the objects appears rehearsed, with no interruptions</li> <li>• Placing the objects does not require alignment movements</li> <li>• No movement is too long; every movement has a clear goal</li> </ul> |

### *Bimanual dexterity*

| 1                                                                                                                                                                                                                                                                                                                                    | 2 | 3                                                                                                                                                                                                                                                                                                                                                                         | 4 | 5                                                                                                                                                                                                                                                                                                                                                                                        |
|--------------------------------------------------------------------------------------------------------------------------------------------------------------------------------------------------------------------------------------------------------------------------------------------------------------------------------------|---|---------------------------------------------------------------------------------------------------------------------------------------------------------------------------------------------------------------------------------------------------------------------------------------------------------------------------------------------------------------------------|---|------------------------------------------------------------------------------------------------------------------------------------------------------------------------------------------------------------------------------------------------------------------------------------------------------------------------------------------------------------------------------------------|
| <ul style="list-style-type: none"> <li>• An object is picked up by one grasper while the other grasper stays at the opposite side of the pegboard</li> <li>• Only one grasper moves to reach the position for transfer</li> <li>• During the transfer, the graspers do not interact and do not move toward the target peg</li> </ul> |   | <ul style="list-style-type: none"> <li>• An object is picked up by one grasper while the other grasper moves towards the position for transfer</li> <li>• During the transfer, the graspers interact but remain in place and do not move toward the target peg</li> <li>• Objects are placed purposefully, while the grasper used for pick-up remains in place</li> </ul> |   | <ul style="list-style-type: none"> <li>• An object is picked up by one grasper while the other one already waits at the position for transfer</li> <li>• During the transfer, the graspers interact and move toward the target peg</li> <li>• Objects are placed purposefully, while the grasper used for pick-up is already moving back to the opposite side of the pegboard</li> </ul> |

### *Tissue handling*

| 1                                                                                                                                                                                              | 2 | 3                                                                                                                                                                                               | 4 | 5                                                                                                                                                                                                                                       |
|------------------------------------------------------------------------------------------------------------------------------------------------------------------------------------------------|---|-------------------------------------------------------------------------------------------------------------------------------------------------------------------------------------------------|---|-----------------------------------------------------------------------------------------------------------------------------------------------------------------------------------------------------------------------------------------|
| <ul style="list-style-type: none"> <li>• Objects are strongly squeezed</li> <li>• Objects are not grasped properly and securely, and without making use of the holes in the objects</li> </ul> |   | <ul style="list-style-type: none"> <li>• Objects are properly grasped and not squeezed</li> <li>• Some pressure is applied to the objects, for example when placing them on the pegs</li> </ul> |   | <ul style="list-style-type: none"> <li>• Objects are properly grasped and not squeezed</li> <li>• Throughout the task, no pressure is applied to the objects, neither when picking them up nor when placing them on the pegs</li> </ul> |

## Circle cutting

### Task description

A two-ply piece of gauze is marked with a circle and secured with four metal clips. Using a grasper and one pair of laparoscopic scissors, the circle must be cut out from the gauze piece, cutting exactly along the marked line. Here, it is irrelevant how much or little of the bottom layer of the gauze is cut. Instruments may be switched between hands at any time.

### Error description

- Cuts are made inside or outside the marked circle.
- The gauze comes out of one (or more) of the metal clips.

### Criteria for exclusion from the dataset

- Task duration > 10 min.
- Gauze is of unsuitable, very coarse material.

### Rating scale with anchor descriptors

#### Depth perception

| 1                                                                                                                                                                                                                                                                                                              | 2 | 3                                                                                                                                                                                                                                                | 4 | 5                                                                                                                                                                                                                                                                                     |
|----------------------------------------------------------------------------------------------------------------------------------------------------------------------------------------------------------------------------------------------------------------------------------------------------------------|---|--------------------------------------------------------------------------------------------------------------------------------------------------------------------------------------------------------------------------------------------------|---|---------------------------------------------------------------------------------------------------------------------------------------------------------------------------------------------------------------------------------------------------------------------------------------|
| <ul style="list-style-type: none"><li>• At the beginning, the gauze must be grasped multiple times to find the starting point</li><li>• The scissors approach slowly and pass the target at least once</li><li>• Cutting motions are repeated because the scissors cut the air rather than the gauze</li></ul> |   | <ul style="list-style-type: none"><li>• The grasper reaches the gauze slowly but steadily</li><li>• In more than half of the cases, the scissors actually cut the gauze</li><li>• The repositioning of the grasper is slow but precise</li></ul> |   | <ul style="list-style-type: none"><li>• At the beginning, scissors and grasper purposefully reach the gauze immediately</li><li>• The gauze is cut with every closure of the scissors</li><li>• Repositioning of the grasper works quickly and without the need to readjust</li></ul> |

#### Efficiency

| 1                                                                                                                                                                                                                                                                                    | 2 | 3                                                                                                                                                                                                                                                                                                                   | 4 | 5                                                                                                                                                                                                                                                                                                                         |
|--------------------------------------------------------------------------------------------------------------------------------------------------------------------------------------------------------------------------------------------------------------------------------------|---|---------------------------------------------------------------------------------------------------------------------------------------------------------------------------------------------------------------------------------------------------------------------------------------------------------------------|---|---------------------------------------------------------------------------------------------------------------------------------------------------------------------------------------------------------------------------------------------------------------------------------------------------------------------------|
| <ul style="list-style-type: none"><li>• At the beginning, the gauze must be grasped multiple times to find the starting point</li><li>• The scissors are not properly aligned and need to be re-aligned multiple times</li><li>• Cuts are made repeatedly at the same spot</li></ul> |   | <ul style="list-style-type: none"><li>• The gauze is reached slowly but steadily</li><li>• The starting point of the cut is maintained; it is avoided to create multiple new starting points</li><li>• Progress is made with more than half of the cuts</li><li>• The grasper is used in a supportive way</li></ul> |   | <ul style="list-style-type: none"><li>• The gauze is reached quickly with both instruments</li><li>• The starting point of the cut is defined with the first cut and is maintained afterward</li><li>• Progress is made with every cut</li><li>• Repositioning of the instruments is deliberate and intentional</li></ul> |

### *Bimanual dexterity*

| 1                                                                                                                                                                                                                                                                                                                                                        | 2 | 3                                                                                                                                                                                                                                                                                                                                                                          | 4 | 5                                                                                                                                                                                                                                                                                                                                                                                 |
|----------------------------------------------------------------------------------------------------------------------------------------------------------------------------------------------------------------------------------------------------------------------------------------------------------------------------------------------------------|---|----------------------------------------------------------------------------------------------------------------------------------------------------------------------------------------------------------------------------------------------------------------------------------------------------------------------------------------------------------------------------|---|-----------------------------------------------------------------------------------------------------------------------------------------------------------------------------------------------------------------------------------------------------------------------------------------------------------------------------------------------------------------------------------|
| <ul style="list-style-type: none"> <li>• The instruments move only one after the other</li> <li>• The grasper does not follow up on time to assist the scissors</li> <li>• The grasper is barely used to support the cutting process and/or interferes with the scissors</li> <li>• The instruments are switched between hands multiple times</li> </ul> |   | <ul style="list-style-type: none"> <li>• Scissors and grasper assist each other and stay close to one another</li> <li>• The grasper does not interfere with the scissors</li> <li>• The grasper follows up to enable the scissors to work effectively, but moves with a delay</li> <li>• The instruments are switched between hands only when it is reasonable</li> </ul> |   | <ul style="list-style-type: none"> <li>• Both instruments move simultaneously, quickly, and purposefully</li> <li>• The grasper follows up as soon as the scissors can no longer cut the gauze easily</li> <li>• The grasper pulls the gauze in the correct direction even from difficult positions</li> <li>• The instruments are switched between hands at most once</li> </ul> |

### *Tissue handling*

| 1                                                                                                                                                                                                                                                                                                            | 2 | 3                                                                                                                                                                                                                                | 4 | 5                                                                                                                                                                                                                 |
|--------------------------------------------------------------------------------------------------------------------------------------------------------------------------------------------------------------------------------------------------------------------------------------------------------------|---|----------------------------------------------------------------------------------------------------------------------------------------------------------------------------------------------------------------------------------|---|-------------------------------------------------------------------------------------------------------------------------------------------------------------------------------------------------------------------|
| <ul style="list-style-type: none"> <li>• The first grip is rough and creates tension on the gauze</li> <li>• The gauze is torn; the grasper tears fibers</li> <li>• Strong tension on the gauze causes it to be pulled out of one of the metal clips</li> <li>• The circle is cut out imprecisely</li> </ul> |   | <ul style="list-style-type: none"> <li>• The gauze does not tear; the fibers remain intact</li> <li>• Some tension is applied to the gauze while gripping</li> <li>• The circle is cut out with some minor deviations</li> </ul> |   | <ul style="list-style-type: none"> <li>• No unnecessary tension is applied to the gauze; fibers are not torn</li> <li>• The circle is cut out precisely</li> <li>• The depth of the cuts is consistent</li> </ul> |

## Balloon resection

### Task description

A standard latex balloon, filled with water, is inserted into another balloon that is marked with a line in reverse T shape. Both balloons are closed with a common knot and mounted with a metal clip at the knotted end. The inner balloon must be removed unbroken from the outer balloon by accurately cutting only the outer layer along the marked line. Instruments may be switched between hands at any time.

### Error description

- Cuts deviate from the marked line.
- The marked line is not completely cut.
- The inner balloon is opened, which means that more than half of the water leaks out. If the inner balloon is opened with the first cut already, the task should be marked as *failed*.
- The inner balloon is damaged, but no more than half of the water leaks out.
- The inner balloon is perforated, which means that only single drops of water leak out or water only leaks out when pressure is applied to the balloon.

### Criteria for exclusion from the dataset

- Task duration > 10 min.
- Light of endoscope is set to low.

### Rating scale with anchor descriptors

| Depth perception                                                                                                                                                                                                                                                                           |   |                                                                                                                                                                                                                                                     |   |                                                                                                                                                                                                                                                                                                                                                                                            |
|--------------------------------------------------------------------------------------------------------------------------------------------------------------------------------------------------------------------------------------------------------------------------------------------|---|-----------------------------------------------------------------------------------------------------------------------------------------------------------------------------------------------------------------------------------------------------|---|--------------------------------------------------------------------------------------------------------------------------------------------------------------------------------------------------------------------------------------------------------------------------------------------------------------------------------------------------------------------------------------------|
| 1                                                                                                                                                                                                                                                                                          | 2 | 3                                                                                                                                                                                                                                                   | 4 | 5                                                                                                                                                                                                                                                                                                                                                                                          |
| <ul style="list-style-type: none"><li>• Multiple attempts are required to grasp the balloons</li><li>• The scissors approach slowly; the first cut is made only after several attempts</li><li>• Very slowly, the scissors are re-aligned with the cutting plane before each cut</li></ul> |   | <ul style="list-style-type: none"><li>• The balloons are grasped purposefully but slowly</li><li>• The scissors approach slowly but steadily</li><li>• After some initial probing, the first cut is successful and is performed with care</li></ul> |   | <ul style="list-style-type: none"><li>• The balloons are grasped quickly; the outer layer is immediately placed under tension to detach the inner balloon</li><li>• The scissors approach immediately, making the first cut quickly and purposefully</li><li>• The scissors remain in the correct cutting plane</li><li>• Repositioning of both instruments is quick and precise</li></ul> |

### *Efficiency*

| 1                                                                                                                                                                                                                                                                                                                                                 | 2 | 3                                                                                                                                                                                                                                                                                                  | 4 | 5                                                                                                                                                                                                                                                                                                  |
|---------------------------------------------------------------------------------------------------------------------------------------------------------------------------------------------------------------------------------------------------------------------------------------------------------------------------------------------------|---|----------------------------------------------------------------------------------------------------------------------------------------------------------------------------------------------------------------------------------------------------------------------------------------------------|---|----------------------------------------------------------------------------------------------------------------------------------------------------------------------------------------------------------------------------------------------------------------------------------------------------|
| <ul style="list-style-type: none"> <li>Multiple attempts are required to grasp the balloons at the beginning</li> <li>The opening in the outer layer is lost during cutting, meaning that the cutting plane must be reestablished</li> <li>The grasper does not support the scissors</li> <li>The scissors are repositioned very often</li> </ul> |   | <ul style="list-style-type: none"> <li>Fewer than two attempts are required to grasp the balloons at the beginning</li> <li>The grasper assists before each cut</li> <li>Cutting the outer layer appears smooth</li> <li>The overall procedure appears fluid, with no noticeable pauses</li> </ul> |   | <ul style="list-style-type: none"> <li>The balloons are grasped only once at the beginning; the outer layer is opened with the first cut</li> <li>The grasper holds the cutting plane in place before each cut</li> <li>The scissors cut continuously without having to be repositioned</li> </ul> |

### *Bimanual dexterity*

| 1                                                                                                                                                                                                                             | 2 | 3                                                                                                                                                                                                                                                                                                                    | 4 | 5                                                                                                                                                                                                                                                                                                                  |
|-------------------------------------------------------------------------------------------------------------------------------------------------------------------------------------------------------------------------------|---|----------------------------------------------------------------------------------------------------------------------------------------------------------------------------------------------------------------------------------------------------------------------------------------------------------------------|---|--------------------------------------------------------------------------------------------------------------------------------------------------------------------------------------------------------------------------------------------------------------------------------------------------------------------|
| <ul style="list-style-type: none"> <li>The second hand does not help to stabilize the balloons for the initial grasp</li> <li>The grasper does not support the cutting process and/or interferes with the scissors</li> </ul> |   | <ul style="list-style-type: none"> <li>The second hand slowly helps to stabilize the balloons for the initial grasp</li> <li>The grasper supports most of the cutting process, staying in contact with the outer layer at least half of the time</li> <li>The grasper rarely interferes with the scissors</li> </ul> |   | <ul style="list-style-type: none"> <li>The second hand quickly helps to stabilize the balloons for the initial grasp</li> <li>The grasper continuously supports the cutting process, staying in contact with the outer layer most of the time</li> <li>The grasper does not interfere with the scissors</li> </ul> |

### *Tissue handling*

| 1                                                                                                                                                                                                                                                                                                                                                                              | 2 | 3                                                                                                                                                                                                                                                                                       | 4 | 5                                                                                                                                                                                                                                                                                                                                                                                                                     |
|--------------------------------------------------------------------------------------------------------------------------------------------------------------------------------------------------------------------------------------------------------------------------------------------------------------------------------------------------------------------------------|---|-----------------------------------------------------------------------------------------------------------------------------------------------------------------------------------------------------------------------------------------------------------------------------------------|---|-----------------------------------------------------------------------------------------------------------------------------------------------------------------------------------------------------------------------------------------------------------------------------------------------------------------------------------------------------------------------------------------------------------------------|
| <ul style="list-style-type: none"> <li>The initial grasp is rough, without careful exposure of the outer layer</li> <li>The outer layer is torn open several times by excessive tension</li> <li>The outer layer is cut roughly and without respecting the marked line</li> <li>The inner balloon is opened, which means that more than half of the water leaks out</li> </ul> |   | <ul style="list-style-type: none"> <li>The initial grasp is gentle</li> <li>The first cut is made after tension is applied to the outer layer to detach the inner balloon</li> <li>The outer layer is not torn</li> <li>Most of the cuts do not deviate from the marked line</li> </ul> |   | <ul style="list-style-type: none"> <li>The outer layer is safely and visibly separated from the inner layer using fine, careful tension by the grasper</li> <li>The first cut is very delicate and minimally opens the outer layer</li> <li>The grasper applies well-controlled tension to the outer layer</li> <li>The cuts do not deviate from the marked line</li> <li>The inner balloon is not damaged</li> </ul> |

## Laparoscopic suture and knot

### Task description

A Penrose drain with a slit and a marked dot on each side of the slit is secured on a Velcro strip. The slit in the Penrose drain must be closed by placing a suture of length 15 cm accurately through the two marked dots and tying a knot. The knot must consist of one double throw, followed by two single throws. The laparoscopic instruments provided for this task are one needle driver to hold the needle end of the suture and one grasper.

*Note:* The maximum time to complete this task is 10 min, which means that the video recording stops after 10 min.

### Error description

- The needle is dropped.
- The suture deviates from any of the two marked dots on the Penrose drain.
- Within 10 min, fewer than three throws are successfully completed. In this case, the task should be marked as *failed*.
- The slit in the Penrose drain is not closed properly.
- The knot slips or comes apart.
- The Penrose drain is separated from the Velcro strip.

### Criteria for exclusion from the dataset

- Within 10 min, no throw can be completed.

### Rating scale with anchor descriptors

#### Depth perception

| 1                                                                                                                                                                                                                                                          | 2 | 3                                                                                                                                                                                                                                                                | 4 | 5                                                                                                                                                                                                                                                                                                                                   |
|------------------------------------------------------------------------------------------------------------------------------------------------------------------------------------------------------------------------------------------------------------|---|------------------------------------------------------------------------------------------------------------------------------------------------------------------------------------------------------------------------------------------------------------------|---|-------------------------------------------------------------------------------------------------------------------------------------------------------------------------------------------------------------------------------------------------------------------------------------------------------------------------------------|
| <ul style="list-style-type: none"><li>• Grasping needle or thread takes multiple attempts</li><li>• The needle approaches the Penrose drain very slowly and misses the marked dots</li><li>• Creating loops of thread requires multiple attempts</li></ul> |   | <ul style="list-style-type: none"><li>• Needle and thread are grasped slowly but reliably</li><li>• The needle approaches the Penrose drain slowly, but hits the marked dots</li><li>• Creating loops of thread is slow but requires only few attempts</li></ul> |   | <ul style="list-style-type: none"><li>• Needle and thread are grasped quickly and reliably</li><li>• The needle is pushed directly through the marked dots, with no corrective movements</li><li>• Loops of thread are created flawlessly and purposefully</li><li>• Loops are tightened precisely, without readjustments</li></ul> |

#### Efficiency

| 1                                                                                                                                                                                                                                                                    | 2 | 3                                                                                                                                                             | 4 | 5                                                                                                                                                                                                                                                                                                                                       |
|----------------------------------------------------------------------------------------------------------------------------------------------------------------------------------------------------------------------------------------------------------------------|---|---------------------------------------------------------------------------------------------------------------------------------------------------------------|---|-----------------------------------------------------------------------------------------------------------------------------------------------------------------------------------------------------------------------------------------------------------------------------------------------------------------------------------------|
| <ul style="list-style-type: none"><li>• The needle must be regrasped or reoriented before stitching</li><li>• After stitching, the needle is grasped incorrectly and must be reoriented</li><li>• The needle is passed between instruments very frequently</li></ul> |   | <ul style="list-style-type: none"><li>• The needle only requires minor adjustments before stitching</li><li>• Stitching is done slowly but steadily</li></ul> |   | <ul style="list-style-type: none"><li>• The needle does not need to be reoriented before stitching</li><li>• Stitching into and out of the Penrose drain can be done in one movement without correction</li><li>• The grasper takes over the needle immediately after stitching, and the first throw can be started instantly</li></ul> |

### *Bimanual dexterity*

| 1                                                                                                                                                                                                                                                                                                                                                                                                      | 2 | 3                                                                                                                                                                                                                                                                                                                                                                      | 4 | 5                                                                                                                                                                                                                                                                                                                                                                                                                                                  |
|--------------------------------------------------------------------------------------------------------------------------------------------------------------------------------------------------------------------------------------------------------------------------------------------------------------------------------------------------------------------------------------------------------|---|------------------------------------------------------------------------------------------------------------------------------------------------------------------------------------------------------------------------------------------------------------------------------------------------------------------------------------------------------------------------|---|----------------------------------------------------------------------------------------------------------------------------------------------------------------------------------------------------------------------------------------------------------------------------------------------------------------------------------------------------------------------------------------------------------------------------------------------------|
| <ul style="list-style-type: none"> <li>• Only one instrument is used to orient the needle</li> <li>• The grasper does not grab the Penrose drain for better visualization of the marked dots</li> <li>• The needle driver both pushes the needle through and pulls the needle out of the Penrose drain; the grasper is not used at all</li> <li>• The instruments interfere with each other</li> </ul> |   | <ul style="list-style-type: none"> <li>• One instrument primarily performs the orientation of the needle; the second one assists only occasionally</li> <li>• During stitching, the grasper takes over only after the motion of the needle driver is finished</li> <li>• When throwing the thread, only one instrument moves while the other remains static</li> </ul> |   | <ul style="list-style-type: none"> <li>• Both instruments assist in orienting the needle</li> <li>• The grasper grabs the Penrose drain to visualize the marked dots</li> <li>• During stitching, the needle driver rotates the needle to a position where the grasper can take over directly</li> <li>• When throwing the thread, both instruments move together</li> <li>• Both instruments interact to pass the needle between hands</li> </ul> |

### *Tissue handling*

| 1                                                                                                                                                                                                                                                                                                                   | 2 | 3                                                                                                                                                                                                                                                                                       | 4 | 5                                                                                                                                                                                                                                                                                                                               |
|---------------------------------------------------------------------------------------------------------------------------------------------------------------------------------------------------------------------------------------------------------------------------------------------------------------------|---|-----------------------------------------------------------------------------------------------------------------------------------------------------------------------------------------------------------------------------------------------------------------------------------------|---|---------------------------------------------------------------------------------------------------------------------------------------------------------------------------------------------------------------------------------------------------------------------------------------------------------------------------------|
| <ul style="list-style-type: none"> <li>• When orienting the needle, the needle is bent and/or the thread is torn</li> <li>• The needle is pushed straight through the tissue instead of being rotated in a semicircular motion</li> <li>• The Penrose drain is damaged when the thread is pulled through</li> </ul> |   | <ul style="list-style-type: none"> <li>• The needle is oriented with little force and little tension on the thread</li> <li>• The Penrose drain is briefly under tension, with little tearing of the material</li> <li>• Loops are tightened forcefully but with low tension</li> </ul> |   | <ul style="list-style-type: none"> <li>• When orienting the needle, the needle is not bent and the thread is not torn</li> <li>• The Penrose drain experiences minimal tension during stitching and no tearing when the thread is pulled through</li> <li>• Loops are tightened without tearing or excessive tension</li> </ul> |
